# Supplementary material for: PIZZA: A Powerful Image-only Zero-Shot Zero-CAD Approach to 6 DoF Tracking
Source: arXiv:2209.07589 source file (2022-10-01)
Supplement: Supplementary file 1 [file supp_qualitative_shapeNet.tex]

\begin{figure}[!t]
\newlength{\qualmodelnetheight}
\setlength\qualmodelnetheight{1.6cm}
\begin{center}
\begin{tabular}{cccccc}
 \includegraphics[ height=\qualmodelnetheight, width=\qualmodelnetheight]{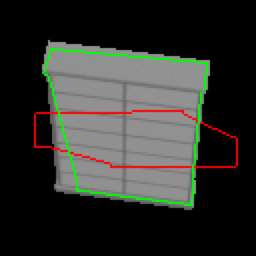} &
 \includegraphics[ height=\qualmodelnetheight, width=\qualmodelnetheight]{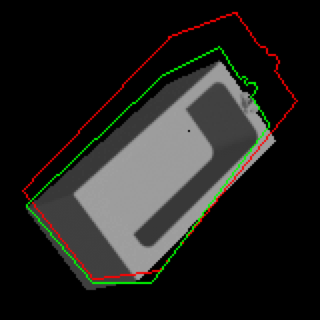} &
 \includegraphics[ height=\qualmodelnetheight, width=\qualmodelnetheight]{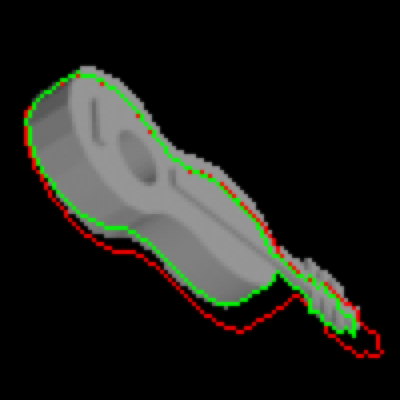} &
 \includegraphics[ height=\qualmodelnetheight, width=\qualmodelnetheight]{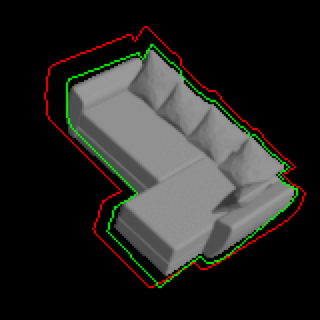}&
 \includegraphics[ height=\qualmodelnetheight, width=\qualmodelnetheight]{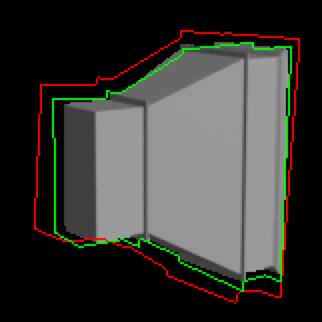} &
 \includegraphics[ height=\qualmodelnetheight, width=\qualmodelnetheight]{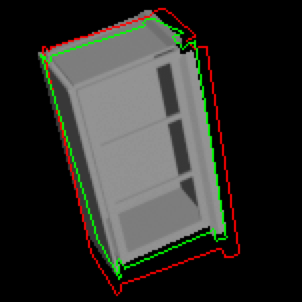}
\end{tabular}\\
\begin{tabular}{cccccc}
 \includegraphics[ height=\qualmodelnetheight, width=\qualmodelnetheight]{images/experiments/modelNet/bookshelf0.png} &
 \includegraphics[ height=\qualmodelnetheight, width=\qualmodelnetheight]{images/experiments/modelNet/bathtub0.png} &
 \includegraphics[ height=\qualmodelnetheight, width=\qualmodelnetheight]{images/experiments/modelNet/guitar1.png} &
 \includegraphics[ height=\qualmodelnetheight, width=\qualmodelnetheight]{images/experiments/modelNet/sofa0.png}&
 \includegraphics[ height=\qualmodelnetheight, width=\qualmodelnetheight]{images/experiments/modelNet/rangehood0.png} &
 \includegraphics[ height=\qualmodelnetheight, width=\qualmodelnetheight]{images/experiments/modelNet/tvstand0.png}
\end{tabular}\\
\begin{tabular}{cccccc}
 \includegraphics[ height=\qualmodelnetheight, width=\qualmodelnetheight]{images/experiments/modelNet/bookshelf0.png} &
 \includegraphics[ height=\qualmodelnetheight, width=\qualmodelnetheight]{images/experiments/modelNet/bathtub0.png} &
 \includegraphics[ height=\qualmodelnetheight, width=\qualmodelnetheight]{images/experiments/modelNet/guitar1.png} &
 \includegraphics[ height=\qualmodelnetheight, width=\qualmodelnetheight]{images/experiments/modelNet/sofa0.png}&
 \includegraphics[ height=\qualmodelnetheight, width=\qualmodelnetheight]{images/experiments/modelNet/rangehood0.png} &
 \includegraphics[ height=\qualmodelnetheight, width=\qualmodelnetheight]{images/experiments/modelNet/tvstand0.png}
\end{tabular}\\
\end{center}
\vspace{-3mm}
\caption{\textbf{Qualitative results on ShapeNet. } We ... }
\label{fig:modelnet_qualitative_results}
\end{figure}
